# Supplementary material for: Dispersed, condensed and self-limiting states of geometrically frustrated assembly
Source: arXiv:2303.02121 ancillary file (2023-08-05)
Supplement: Supplementary file 1 [file Hackney_2023_SI.pdf]

# Supplemental Information for Dispersed, Condensed and Self-Limiting States of Geometrically Frustrated Assembly

Nicholas W. Hackney

*Department of Physics, University of Massachusetts Amherst*

Chris Amey

*Department of Physics, Brandeis University*

Gregory M. Grason

*Department of Polymer Science and Engineering, University of Massachusetts Amherst\**

---

\*Electronic address: [grason@umass.edu](mailto:grason@umass.edu)

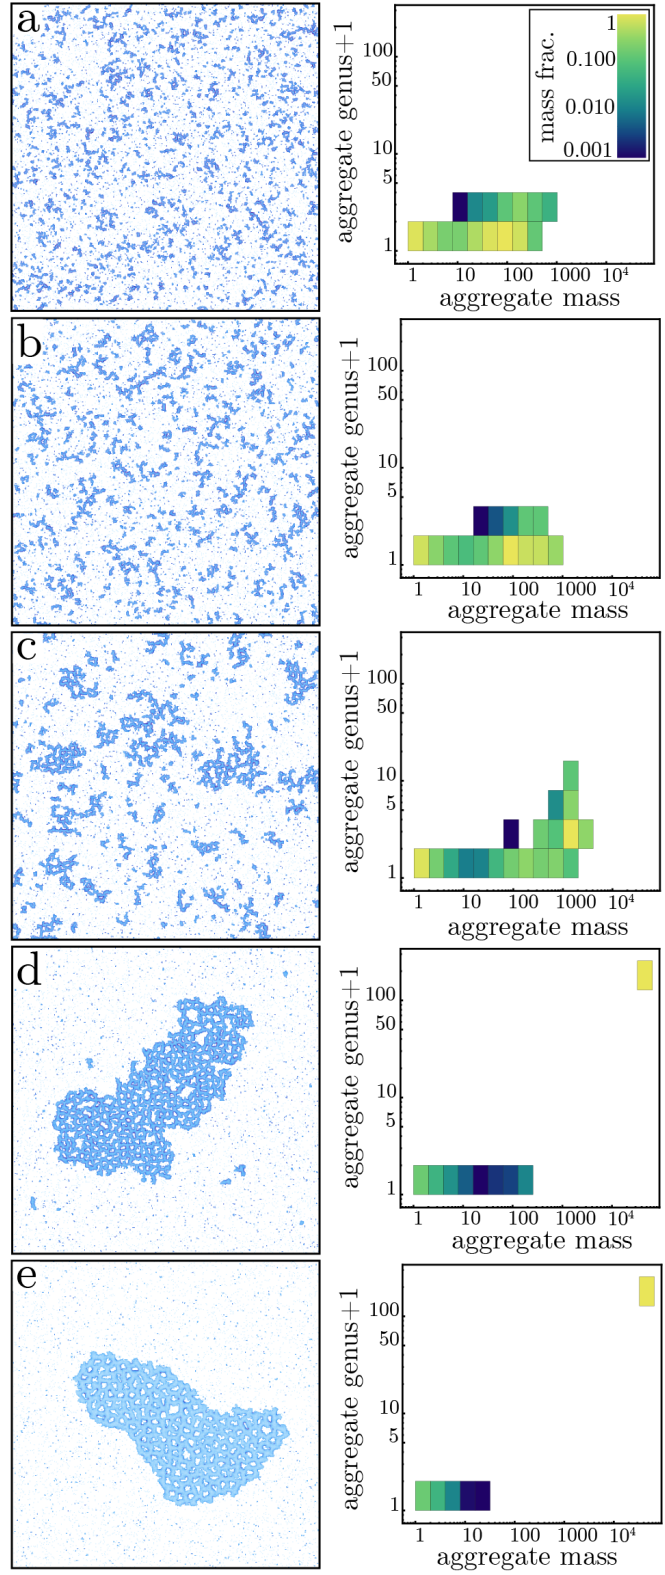

FIG. S1: **Concentration of Sub-units by Aggregate Size and Topology** The mass distribution of sub-units as a function of aggregate size and topology for a range of frustrations sweeping across the condensation transition. The distributions are given for the  $\Phi = 0.18$  column of the visual phase diagram shown in Figure 10 of the main text and the following values of frustration: **a)**  $f = 0.020$  **b)**  $f = 0.016$  **c)**  $f = 0.012$  **d)**  $f = 0.008$  **e)**  $f = 0.004$ . The full  $500 \times 500$  lattice is shown for each simulation; this is in contrast to the  $150 \times 150$  subsets given in Fig. 10. Here we can see that, while the poly-disperse self-limiting aggregates (a-c) become increasingly loopy as the critical frustration is approached, the condensed bulk phase (d-e) can be differentiated by their (quasi) bi-disperse mass distribution. The mass/genus distributions shown here are taken from a single simulation snapshot and do not represent time averaged values obtained from many statistically independent samples. Finally, The genus of each aggregate was incremented by one to allow aggregates with zero holes to be plotted on a log scale.

| MC simulation parameters for Main Text Figure 1 |       |           |        |     |                |  |
|-------------------------------------------------|-------|-----------|--------|-----|----------------|--|
| $\Sigma/J$                                      | $f$   | $\beta J$ | $\Phi$ | $L$ | $N_s$          |  |
| 0.09                                            | 0.012 | 40        | 0.02   | 500 | $5 \cdot 10^6$ |  |
| 0.09                                            | 0.012 | 40        | 0.08   | 500 | $5 \cdot 10^6$ |  |
| 0.09                                            | 0.004 | 40        | 0.08   | 500 | $5 \cdot 10^6$ |  |

TABLE S1: Parameters for example states of assembly

| MC simulation parameters for Main Text Figure 3 |            |       |           |        |     |                |
|-------------------------------------------------|------------|-------|-----------|--------|-----|----------------|
| phase                                           | $\Sigma/J$ | $f$   | $\beta J$ | $\Phi$ | $L$ | $N_s$          |
| dispersed                                       | 0.09       | 0     | 40        | 0.02   | 500 | $5 \cdot 10^6$ |
| droplet                                         | 0.09       | 0     | 40        | 0.04   | 500 | $5 \cdot 10^6$ |
| redispersed                                     | 0.09       | 0.012 | 40        | 0.04   | 500 | $5 \cdot 10^6$ |
| aggregated                                      | 0.09       | 0.012 | 40        | 0.08   | 500 | $5 \cdot 10^6$ |

TABLE S2: Parameters for sequence illustrating affect of concentration and frustration on assembly

| MC simulation parameters for Main Text Figure 4b and inset of 6a |            |       |           |        |     |                |
|------------------------------------------------------------------|------------|-------|-----------|--------|-----|----------------|
| Line color                                                       | $\Sigma/J$ | $f$   | $\beta J$ | $\Phi$ | $L$ | $N_s$          |
| Black                                                            | 0.09       | 0.016 | 40        | 0.04   | 500 | $5 \cdot 10^6$ |
| Purple                                                           | 0.09       | 0.016 | 40        | 0.06   | 500 | $5 \cdot 10^6$ |
| Blue                                                             | 0.09       | 0.016 | 40        | 0.08   | 500 | $5 \cdot 10^6$ |
| Green                                                            | 0.09       | 0.016 | 40        | 0.012  | 500 | $5 \cdot 10^6$ |
| Orange                                                           | 0.09       | 0.016 | 40        | 0.016  | 500 | $5 \cdot 10^6$ |
| Red                                                              | 0.09       | 0.016 | 40        | 0.022  | 500 | $5 \cdot 10^6$ |

TABLE S3: Parameters for measuring aggregate mass and width distribution for increasing concentration

| MC simulation parameters for Main Text Figure 5 and 7 |        |           |        |      |                |
|-------------------------------------------------------|--------|-----------|--------|------|----------------|
| $\Sigma/J$                                            | $f$    | $\beta J$ | $\Phi$ | $L$  | $N_s$          |
| 0.09                                                  | 0.015  | 40        | 0.3    | 800  | $5 \cdot 10^6$ |
| 0.005                                                 | 0.0015 | 650       | 0.30   | 4000 | $5 \cdot 10^5$ |
| 0.005                                                 | 0.001  | 650       | 0.30   | 4000 | $5 \cdot 10^5$ |
| 0.005                                                 | 0.0005 | 650       | 0.30   | 4000 | $5 \cdot 10^5$ |

TABLE S4: Parameters for looking at branched vs. linear aggregate behavior at large  $n$  as well as investigating the compact to extended morphology transition.

| MC simulation parameters for Main Text Figure 6b |            |               |            |           |        |      |                |
|--------------------------------------------------|------------|---------------|------------|-----------|--------|------|----------------|
| Symbol                                           | $\Sigma/J$ | $f$           | $\Delta f$ | $\beta J$ | $\Phi$ | $L$  | $N_s$          |
| ○                                                | 0.09       | 0.0075-0.05   | 0.0025     | 40        | 0.2    | 800  | $5 \cdot 10^6$ |
| ●                                                | 0.005      | 0.0005-0.0025 | 0.0005     | 650       | 0.3    | 4000 | $5 \cdot 10^5$ |
| ■                                                | 0.01       | 0.0005-0.0025 | 0.0005     | 325       | 0.16   | 1000 | $10^5$         |
| □                                                | 0.05       | 0.0025-0.025  | 0.0025     | 72        | 0.15   | 800  | $10^6$         |
| ▲                                                | 0.2        | 0.015-0.07    | 0.0025     | 18        | 0.15   | 800  | $2 \cdot 10^6$ |

TABLE S5: Parameters for investigating affect of frustration on self-limiting aggregation width.

| MC simulation parameters for Main Text Figure 8 |            |         |            |           |          |              |     |                  |
|-------------------------------------------------|------------|---------|------------|-----------|----------|--------------|-----|------------------|
| Symbol                                          | $\Sigma/J$ | $f$     | $\Delta f$ | $\beta J$ | $\Phi$   | $\Delta\Phi$ | $L$ | $N_s$            |
| ■                                               | 0.05       | 0-0.04  | 0.004      | 72        | 0.02-0.4 | 0.02         | 500 | $2 \cdot 10^6$   |
| ●                                               | 0.09       | 0-0.04  | 0.004      | 40        | 0.02-0.4 | 0.02         | 500 | $2.5 \cdot 10^6$ |
| ○                                               | 0.09       | 0-0.1   | 0.004      | 45        | 0.02-0.4 | 0.02         | 500 | $3 \cdot 10^6$   |
| ◆                                               | 0.15       | 0-0.032 | 0.004      | 24        | 0.01-0.3 | 0.01         | 500 | $3 \cdot 10^6$   |

TABLE S6: Parameters for critical aggregation contour shown in 2D SLA Phase diagram.

| MC simulation parameters for Main Text Figure 9a |        |           |        |     |                  |  |
|--------------------------------------------------|--------|-----------|--------|-----|------------------|--|
| $\Sigma/J$                                       | $f$    | $\beta J$ | $\Phi$ | $L$ | $N_s$            |  |
| 0.09                                             | 0.0025 | 40        | 0.15   | 800 | $1.5 \cdot 10^6$ |  |
| 0.09                                             | 0.0075 | 40        | 0.15   | 800 | $1.5 \cdot 10^6$ |  |
| 0.09                                             | 0.0125 | 40        | 0.15   | 800 | $1.5 \cdot 10^6$ |  |
| 0.09                                             | 0.0225 | 40        | 0.15   | 800 | $1.5 \cdot 10^6$ |  |

  

| MC simulation parameters for finite-size scaling in Main Text Figure 9b |            |             |           |        |          |            |                |
|-------------------------------------------------------------------------|------------|-------------|-----------|--------|----------|------------|----------------|
| Symbol                                                                  | $\Sigma/J$ | $f$         | $\beta J$ | $\Phi$ | $L$      | $\Delta L$ | $N_s$          |
| ●                                                                       | 0.09       | 0           | 40        | 0.15   | 100-1200 | 100        | $5 \cdot 10^6$ |
| ■                                                                       | 0.09       | 0.005       | 40        | 0.15   | 400-1400 | 400        | $5 \cdot 10^6$ |
| ◆                                                                       | 0.09       | 0.008       | 40        | 0.15   | 250-1250 | 250        | $5 \cdot 10^6$ |
| ▲                                                                       | 0.09       | 0.01        | 40        | 0.15   | 200-1200 | 200        | $5 \cdot 10^6$ |
| ▼                                                                       | 0.09       | 0.0125      | 40        | 0.15   | 160-1120 | 160        | $5 \cdot 10^6$ |
| ○                                                                       | 0.09       | 0.013333333 | 40        | 0.15   | 150-1050 | 150        | $5 \cdot 10^6$ |
| □                                                                       | 0.09       | 0.014285714 | 40        | 0.15   | 140-1120 | 140        | $5 \cdot 10^6$ |
| ◇                                                                       | 0.09       | 0.016       | 40        | 0.15   | 125-1000 | 125        | $5 \cdot 10^6$ |
| △                                                                       | 0.09       | 0.02        | 40        | 0.15   | 100-1000 | 100        | $5 \cdot 10^6$ |

TABLE S7: Parameters for sequence of aggregated states crossing the condensed to self-limiting aggregation transition (top table) and series of simulations with increasing frustration and lattice size for finite size scaling analysis.

| MC simulation parameters for black data of Main Text Fig. 9c                             |             |            |                |           |            |                  |
|------------------------------------------------------------------------------------------|-------------|------------|----------------|-----------|------------|------------------|
| $\Sigma/J$                                                                               | $f$         | $\beta J$  | $\Phi$         | $L$       | $\Delta L$ | $N_s$            |
| 0.05                                                                                     | 0           | 72         | 0.12,0.15,0.20 | 100-1200  | 100        | $3.5 \cdot 10^6$ |
| 0.05                                                                                     | 0.002       | 72         | 0.12,0.15,0.20 | 1000-2000 | 1000       | $3.5 \cdot 10^6$ |
| 0.05                                                                                     | 0.0025      | 72         | 0.12,0.15,0.20 | 800-2400  | 800        | $3.5 \cdot 10^6$ |
| 0.05                                                                                     | 0.004       | 72         | 0.12,0.15,0.20 | 500-2000  | 500        | $3.5 \cdot 10^6$ |
| 0.05                                                                                     | 0.005       | 72         | 0.12,0.15,0.20 | 400-2000  | 400        | $3.5 \cdot 10^6$ |
| 0.05                                                                                     | 0.0075      | 72         | 0.12,0.15,0.20 | 800-1600  | 800        | $3.5 \cdot 10^6$ |
| 0.05                                                                                     | 0.008       | 72         | 0.12,0.15,0.20 | 250-1250  | 250        | $3.5 \cdot 10^6$ |
| 0.05                                                                                     | 0.01        | 72         | 0.12,0.15,0.20 | 200-2000  | 200        | $3.5 \cdot 10^6$ |
| 0.05                                                                                     | 0.0125      | 72         | 0.12,0.15,0.20 | 160-2080  | 0.0125     | $3.5 \cdot 10^6$ |
| MC simulation parameters for green data of Main Text Fig. 9c                             |             |            |                |           |            |                  |
| $\Sigma/J$                                                                               | $f$         | $\beta J$  | $\Phi$         | $L$       | $\Delta L$ | $N_s$            |
| 0.09                                                                                     | 0           | 40         | 0.12,0.15,0.20 | 100-1200  | 100        | $5 \cdot 10^6$   |
| 0.09                                                                                     | 0.005       | 40         | 0.12,0.15,0.20 | 400-1400  | 400        | $5 \cdot 10^6$   |
| 0.09                                                                                     | 0.008       | 40         | 0.12,0.15,0.20 | 250-1250  | 250        | $5 \cdot 10^6$   |
| 0.09                                                                                     | 0.01        | 40         | 0.12,0.15,0.20 | 200-1200  | 200        | $5 \cdot 10^6$   |
| 0.09                                                                                     | 0.0125      | 40         | 0.12,0.15,0.20 | 160-1120  | 160        | $5 \cdot 10^6$   |
| 0.09                                                                                     | 0.013333333 | 40         | 0.12,0.15,0.20 | 150-1050  | 150        | $5 \cdot 10^6$   |
| 0.09                                                                                     | 0.014285714 | 40         | 0.12,0.15,0.20 | 140-1120  | 140        | $5 \cdot 10^6$   |
| 0.09                                                                                     | 0.016       | 40         | 0.12,0.15,0.20 | 125-1000  | 125        | $5 \cdot 10^6$   |
| 0.09                                                                                     | 0.02        | 40         | 0.12,0.15,0.20 | 100-1000  | 100        | $5 \cdot 10^6$   |
| MC simulation parameters for purple data of Main Text Fig. 9c                            |             |            |                |           |            |                  |
| $\Sigma/J$                                                                               | $f$         | $\beta J$  | $\Phi$         | $L$       | $\Delta L$ | $N_s$            |
| 0.2                                                                                      | 0           | 18         | 0.12,0.15,0.20 | 100-1200  | 100        | $3.5 \cdot 10^6$ |
| 0.2                                                                                      | 0.01        | 18         | 0.12,0.15,0.20 | 200-1200  | 200        | $3.5 \cdot 10^6$ |
| 0.2                                                                                      | 0.015       | 18         | 0.12,0.15,0.20 | 125-1250  | 125        | $3.5 \cdot 10^6$ |
| 0.2                                                                                      | 0.02        | 18         | 0.12,0.15,0.20 | 100-1200  | 100        | $3.5 \cdot 10^6$ |
| 0.2                                                                                      | 0.025       | 18         | 0.12,0.15,0.20 | 80-1200   | 80         | $3.5 \cdot 10^6$ |
| 0.2                                                                                      | 0.03125     | 18         | 0.12,0.15,0.20 | 64-1216   | 64         | $3.5 \cdot 10^6$ |
| 0.2                                                                                      | 0.04        | 18         | 0.12,0.15,0.20 | 50-1200   | 50         | $3.5 \cdot 10^6$ |
| Parameters for black, green and purple data (respectively) in Main Text Fig. 9c (bottom) |             |            |                |           |            |                  |
| $\Sigma/J$                                                                               | $f$         | $\Delta f$ | $\beta J$      | $\Phi$    | $L$        | $N_s$            |
| 0.05                                                                                     | 0.0025-0.04 | 0.0025     | 72             | 0.15      | 800        | $10^6$           |
| 0.09                                                                                     | 0.0025-0.04 | 0.0025     | 40             | 0.15      | 800        | $10^6$           |
| 0.2                                                                                      | 0.0025-0.04 | 0.0025     | 18             | 0.15      | 800        | $2.5 \cdot 10^6$ |

TABLE S8: Parameters for measuring topological charge and finite size scaling exponent as frustration is varied from weak to strong.

| MC simulation parameters for black data ( $\beta\Sigma = 3.6$ ) in Main Text Fig. 9d |        |            |           |                |      |                  |
|--------------------------------------------------------------------------------------|--------|------------|-----------|----------------|------|------------------|
| $\Sigma/J$                                                                           | $f$    | $\Delta f$ | $\beta J$ | $\Phi$         | $L$  | $N_s$            |
| 0.05                                                                                 | 0-0.1  | 0.0025     | 72        | 0.1,0.15       | 800  | $10^6$           |
| 0.07                                                                                 | 0-0.1  | 0.0025     | 51.4      | 0.1,0.15       | 800  | $3.2 \cdot 10^6$ |
| 0.09                                                                                 | 0-0.1  | 0.0025     | 40        | 0.15           | 800  | $10^6$           |
| 0.12                                                                                 | 0-0.1  | 0.0025     | 30        | 0.1,0.15       | 800  | $3.2 \cdot 10^6$ |
| 0.2                                                                                  | 0-0.1  | 0.0025     | 18        | 0.1,0.15       | 800  | $2.5 \cdot 10^6$ |
| 0.3                                                                                  | 0-0.1  | 0.0025     | 12        | 0.1,0.15,0.2   | 800  | $2 \cdot 10^6$   |
| 0.5                                                                                  | 0-0.15 | 0.0025     | 7.2       | 0.1,0.2,0.3    | 800  | $2.2 \cdot 10^6$ |
| 0.75                                                                                 | 0-0.2  | 0.0025     | 4.8       | 0.1            | 800  | $3 \cdot 10^6$   |
| 0.875                                                                                | 0-0.2  | 0.0025     | 4.114     | 0.1            | 800  | $5 \cdot 10^5$   |
| 1                                                                                    | 0-0.5  | 0.0025     | 3.6       | 0.15           | 800  | $2.5 \cdot 10^6$ |
| MC simulation parameters for red data ( $\beta\Sigma = 5.4$ ) in Main Text Fig. 9d   |        |            |           |                |      |                  |
| $\Sigma/J$                                                                           | $f$    | $\Delta f$ | $\beta J$ | $\Phi$         | $L$  | $N_s$            |
| 0.025                                                                                | 0-0.05 | 0.02       | 216       | 0.10,0.15      | 1000 | $1.3 \cdot 10^6$ |
| 0.05                                                                                 | 0-0.1  | 0.0025     | 108       | 0.08,0.10,0.12 | 800  | $1.3 \cdot 10^6$ |
| 0.09                                                                                 | 0-0.1  | 0.0025     | 60        | 0.08,0.10,0.12 | 800  | $2.5 \cdot 10^6$ |
| 0.15                                                                                 | 0-0.1  | 0.0025     | 36        | 0.08,0.10,0.12 | 800  | $1.2 \cdot 10^6$ |
| 0.2                                                                                  | 0-0.1  | 0.0025     | 27        | 0.06,0.08,0.10 | 800  | $2.5 \cdot 10^6$ |
| 0.3                                                                                  | 0-0.1  | 0.0025     | 18        | 0.06,0.08,0.1  | 800  | $10^6$           |
| 0.5                                                                                  | 0-0.15 | 0.0025     | 10.8      | 0.08,0.10      | 800  | $10^5$           |
| MC simulation parameters for blue data ( $\beta\Sigma = 7.2$ ) in Main Text Fig. 9d  |        |            |           |                |      |                  |
| $\Sigma/J$                                                                           | $f$    | $\Delta f$ | $\beta J$ | $\Phi$         | $L$  | $N_s$            |
| 0.02                                                                                 | 0-0.05 | 0.001      | 360       | 0.04,0.08      | 2000 | $10^6$           |
| 0.025                                                                                | 0-0.05 | 0.0025     | 288       | 0.08-0.08      | 800  | $3.5 \cdot 10^6$ |
| 0.03                                                                                 | 0-0.05 | 0.0025     | 240       | 0.06,0.08      | 800  | $3.5 \cdot 10^6$ |
| 0.04                                                                                 | 0-0.05 | 0.0025     | 180       | 0.06,0.08      | 800  | $3.5 \cdot 10^6$ |
| 0.05                                                                                 | 0-0.1  | 0.0025     | 144       | 0.06,0.08      | 800  | $2.5 \cdot 10^6$ |
| 0.15                                                                                 | 0-0.15 | 0.0025     | 48        | 0.06,0.08      | 800  | $2 \cdot 10^6$   |

TABLE S9: Simulation parameters for measuring critical value of frustration for several different values of temperature.

| Simulation parameters for the visual phase diagram in Figure 10 |         |            |           |           |              |     |                |
|-----------------------------------------------------------------|---------|------------|-----------|-----------|--------------|-----|----------------|
| $\Sigma/J$                                                      | $f$     | $\Delta f$ | $\beta J$ | $\Phi$    | $\Delta\Phi$ | $L$ | $N_s$          |
| 0.09                                                            | 0-0.032 | 0.004      | 40        | 0.02-0.18 | 0.02         | 500 | $6 \cdot 10^6$ |

TABLE S10: Simulation parameters used to construct the visual phase diagram mosaic.

| Varying frustration                                   |          |                       | Varying concentration                                |          |
|-------------------------------------------------------|----------|-----------------------|------------------------------------------------------|----------|
| $\Sigma/J = 0.05, \Phi = 0.16, \beta J = 72, L = 800$ |          |                       | $\Sigma/J = 0.05, f = 0.015, \beta J = 72, L = 800$  |          |
| $f$                                                   | $\tau_a$ | degree of frustration | $\Phi$                                               | $\tau_a$ |
| 0.0025                                                | 2923     | weak                  | 0.08                                                 | 236      |
| 0.0050                                                | 470      | weak                  | 0.12                                                 | 194      |
| 0.0075                                                | 17       | strong                | 0.16                                                 | 144      |
| 0.0100                                                | 89       | strong                | 0.2                                                  | 130      |
| 0.0125                                                | 126      | strong                | $\Sigma/J = 0.09, f = 0.015, \beta J = 40, L = 800$  |          |
| 0.015                                                 | 174      | strong                | $\Phi$                                               | $\tau_a$ |
| 0.0175                                                | 197      | strong                | 0.08                                                 | 146      |
| 0.0225                                                | 194      | strong                | 0.12                                                 | 69       |
| 0.025                                                 | 192      | strong                | 0.16                                                 | 56       |
| $\Sigma/J = 0.09, \Phi = 0.16, \beta J = 40, L = 800$ |          |                       | 0.2                                                  | 34       |
| $f$                                                   | $\tau_a$ | degree of frustration | $\Sigma/J = 0.20, f = 0.0275, \beta J = 18, L = 800$ |          |
| 0.0025                                                | 2260     | weak                  | $\Phi$                                               | $\tau_a$ |
| 0.005                                                 | 615      | weak                  | 0.04                                                 | 200      |
| 0.0075                                                | 418      | weak                  | 0.08                                                 | 147      |
| 0.01                                                  | 134      | weak                  | 0.12                                                 | 87       |
| 0.0125                                                | 40       | strong                | 0.16                                                 | 60       |
| 0.015                                                 | 62       | strong                |                                                      |          |
| 0.0175                                                | 107      | strong                |                                                      |          |
| 0.02                                                  | 126      | strong                |                                                      |          |
| 0.0225                                                | 156      | strong                |                                                      |          |
| 0.025                                                 | 195      | strong                |                                                      |          |
| $\Sigma/J = 0.20, \Phi = 0.16, \beta J = 18, L = 800$ |          |                       |                                                      |          |
| $f$                                                   | $\tau_a$ | degree of frustration |                                                      |          |
| 0.005                                                 | 4599     | weak                  |                                                      |          |
| 0.0075                                                | 3247     | weak                  |                                                      |          |
| 0.01                                                  | 62       | weak                  |                                                      |          |
| 0.0125                                                | 411      | weak                  |                                                      |          |
| 0.015                                                 | 308      | weak                  |                                                      |          |
| 0.02                                                  | 12       | strong                |                                                      |          |
| 0.0225                                                | 13       | strong                |                                                      |          |
| 0.025                                                 | 42       | strong                |                                                      |          |
| 0.0275                                                | 60       | strong                |                                                      |          |
| 0.03                                                  | 86       | strong                |                                                      |          |
| 0.0325                                                | 100      | strong                |                                                      |          |

TABLE S11: Auto-Correlation times (in units of Monte Carlo sweeps) computed for several different values of  $\Sigma/J$  and  $\beta J$  over a range of concentration and frustration.

### Supplementary Note 1. CONTINUUM LIMIT OF LATTICE MODEL

An analytic function for the ground-state energetics of our rigid worm aggregates can be obtained by solving the Euler-Lagrange equations for our continuum model (Main text eq. 19-20) over fixed rectangular domains of dimension  $X' \times Y'$ , where the ' refers to the number of bonds in the dimension (i.e. less than the number particles by 1). This can be done via a separation of variables, where we look for solutions of the form:  $\theta(x, y) = G(x)H(y)$ . Substituting this into our PDE we obtain two second order homogeneous equations for  $G(x)$  and  $H(y)$  with solutions:

$$\begin{aligned} i) \quad G(x) &= a_0 + b_0x + a_q e^{qx} + b_q e^{-qx} \\ ii) \quad H(y) &= c_0 + d_0y + c_k e^{ky} + d_k e^{-ky} \end{aligned} \quad (S1)$$

where  $q$  and  $k$  are separation constants required to satisfy  $q^2 + k^2 = 0$  and  $a, b, c, d$  are Fourier coefficients. Noting that the requirement placed upon  $q$  and  $k$  suggests that  $q = ik$ , we can now write the entire solution for  $\theta(x, y)$  as:

$$\begin{aligned} \theta(x, y) &= a_0c_0 + a_0d_0y + b_0c_0x + b_0d_0xy \\ &+ \sum_{n=1} (a_n \sin k_n x + b_n \cos k_n x)(c_n e^{k_n y} + d_n e^{-k_n y}) \end{aligned} \quad (S2)$$

In the case of rectangular domains, we find that our boundary conditions (Main Text eq. 20) are satisfied by setting the constants  $a_n = 0$ ,  $a_0d_0 = -\frac{f}{2}X'$ ,  $a_0c_0 = 0$ ,  $b_0c_0 = -\frac{f}{2}Y$ ,  $b_0d_0 = f$  and taking the remaining Fourier coefficient groupings to be:

$$\begin{aligned} b_n c_n &= \frac{1}{1 + e^{k_n Y'}} \frac{\Gamma_n}{k_n} \\ b_n d_n &= \frac{-e^{k_n Y'}}{1 + e^{k_n Y'}} \frac{\Gamma_n}{k_n} \end{aligned} \quad (S3)$$

where we have defined:

$$\begin{aligned} k_n &= \frac{n\pi}{X'} \\ \Gamma_n &= \frac{4fX'}{\pi^2 n^2} \quad \text{for } n = 1, 3, 5, \dots \end{aligned} \quad (S4)$$

We can now write our final solution in the concise form:

$$\theta(x, y) = -\frac{f}{2}X' + \frac{f}{2}xy + \sum_{n \text{ odd}} (c_n e^{k_n y} + d_n e^{-k_n y}) \cos(k_n x) \quad (S5)$$

Substituting this solution back into our continuum Hamiltonian (Main Text eq. 3) and dividing by aggregate area, gives the results in main text eqs. (21) and (22).

### Supplementary Note 2. EFFECTS OF LATTICE CUTOFF

The quantitative effects of the microscopic lattice cutoff on the aggregation behavior of our model can be investigated by retaining the  $X' = X - 1$  and  $Y' = Y - 1$  terms in Main Text eq. 21. Following the Methods, this energy density can be rescaled by the substitutions  $X = \ell_d \bar{X}$  and  $Y = \ell_d \bar{Y}$  and subsequently written as a function of aspect ratio,  $\alpha$ , and dimensionless area,  $\bar{n}$ , via the additional substitution:  $\bar{X} = \sqrt{\alpha \bar{n}}$  and  $\bar{Y} = \sqrt{\bar{n}/\alpha}$ . Doing so, we find:

$$\frac{\epsilon(\alpha, \bar{n})}{\Sigma/\ell_d} = \Omega(\alpha)(\sqrt{\alpha \bar{n}} - 1)^2 + \frac{1}{\sqrt{\bar{n}}} \left( \frac{1}{\sqrt{\alpha}} + \sqrt{\alpha} \right). \quad (S6)$$

Note that, for simplicity (and without noticeable quantitative error) we take  $X'/Y' \rightarrow X/Y$  in argument of  $\Omega$ . The resulting energy density can be minimized with respect to  $\alpha$  to find the aspect ratio minimized energy density as a function of aggregate size  $\epsilon_m(\bar{n}) = \min_{\alpha}[\epsilon(\alpha, \bar{n})]$ . Plotting the energy density minimizing aspect ratio as a function of  $\bar{n}$  (See Fig. S2), for a variety of  $\ell_d^{-1}$ , we see that as the microscopic cutoff becomes small ( $\ell_d^{-1} \rightarrow 0$ ) the ‘‘Pitchfork’’ saddle behavior obtained from the  $(X', Y') \rightarrow (X, Y)$  approximation is reclaimed and that the sharp bifurcation at  $\bar{n}_c$  is a continuous splitting that extends down to finite value of  $\ell_d^{-1}$ . However, as  $\ell_d^{-1} \rightarrow 0$ , the optimal shapes approach

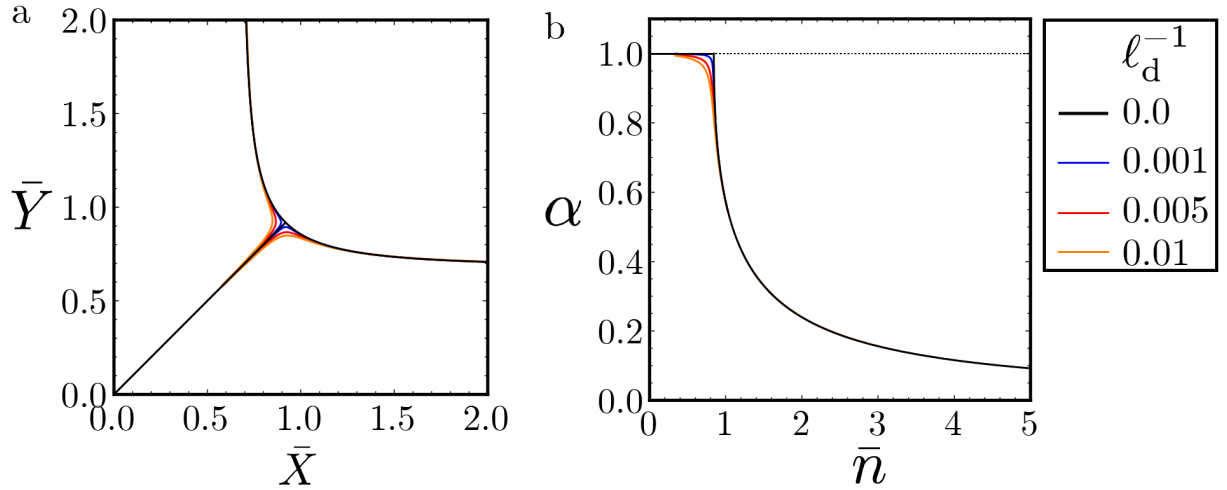

FIG. S2: **Affect of microscopic lattice cutoff on optimal aspect ratio of rectangular aggregates** **a** bifurcated saddle path of minimum energy density rectangular aggregates as function of reduced dimensions  $\bar{X}$  and  $\bar{Y}$  shown for several different values of  $\ell_d^{-1}$ . **b** Energy density minimizing aspect ratio as a function of dimensionless aggregate size  $\bar{n}$  for same sequence of  $\ell_d^{-1}$ .

the singular behavior of the continuum limit. Similarly, the energy density along the aspect ratio minimized “saddle path” approaches the cutoff-free limit as  $\ell_{d-1} \rightarrow 0$  (see Figure S3). Notably,  $\epsilon(1) = 0$  properly only when including the microscopic cutoff, and the  $(X', Y') \rightarrow (X, Y)$  introduces an error to the free monomer energy that decreases as  $\ell_{d-1} \rightarrow 0$ .

Incorporating these calculations into the ideal aggregation theory, we compare mass distributions from the continuum model both with and without including the microscopic cutoff for two different values of frustration Fig. S4. As  $\ell_{d-1} \propto f^{2/3}$  (and the characteristic domain size grows larger for small  $f$ ) decreasing frustration leads to smaller discrepancy between calculations that include and omit the lattice cutoff.

In Fig. S5 we compare the ideal aggregation of rectangular aggregates both with and without the lattice cutoff to the simplified 1D chain approximation of finite-width ribbons described in Methods and used to model aggregation transitions in Main Text Figure 3. We note that results both with and without the cutoff closely follow one another, and while there is an offset relative to the 1D chain approximation, the relative shifts of all three model approximations with increased  $f$  closely match one another. This comparison shows that the predominant dependence of aggregation energetics on frustration is largely independent of microscopic details of at the lattice scale, and instead dominated by features of the large- $n$  tail, a limit at which all three approximations converge.

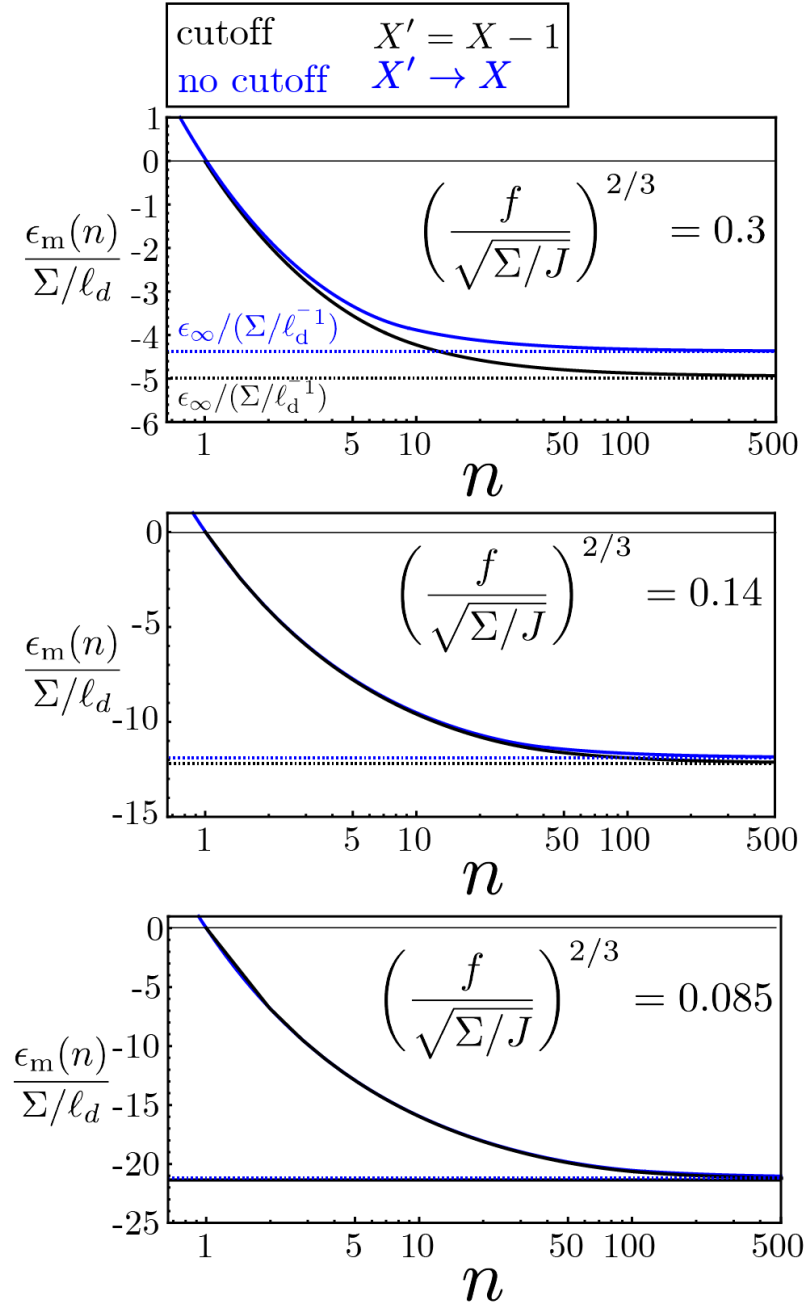

FIG. S3: **Affect of lattice cutoff on per subunit aggregate energy** Comparison of the aspect ratio minimized energy density for several different, decreasing, values of  $\ell_d^{-1}$ . Here we can see that the microscopic cutoff, contrary to the cutoff-free case, appropriately shifts the energy density such that it is equal to zero at  $n = 1$ . Furthermore, we observe that the  $n \rightarrow \infty$  limits of the two theories converge as  $\ell_d^{-1}$  goes to zero.

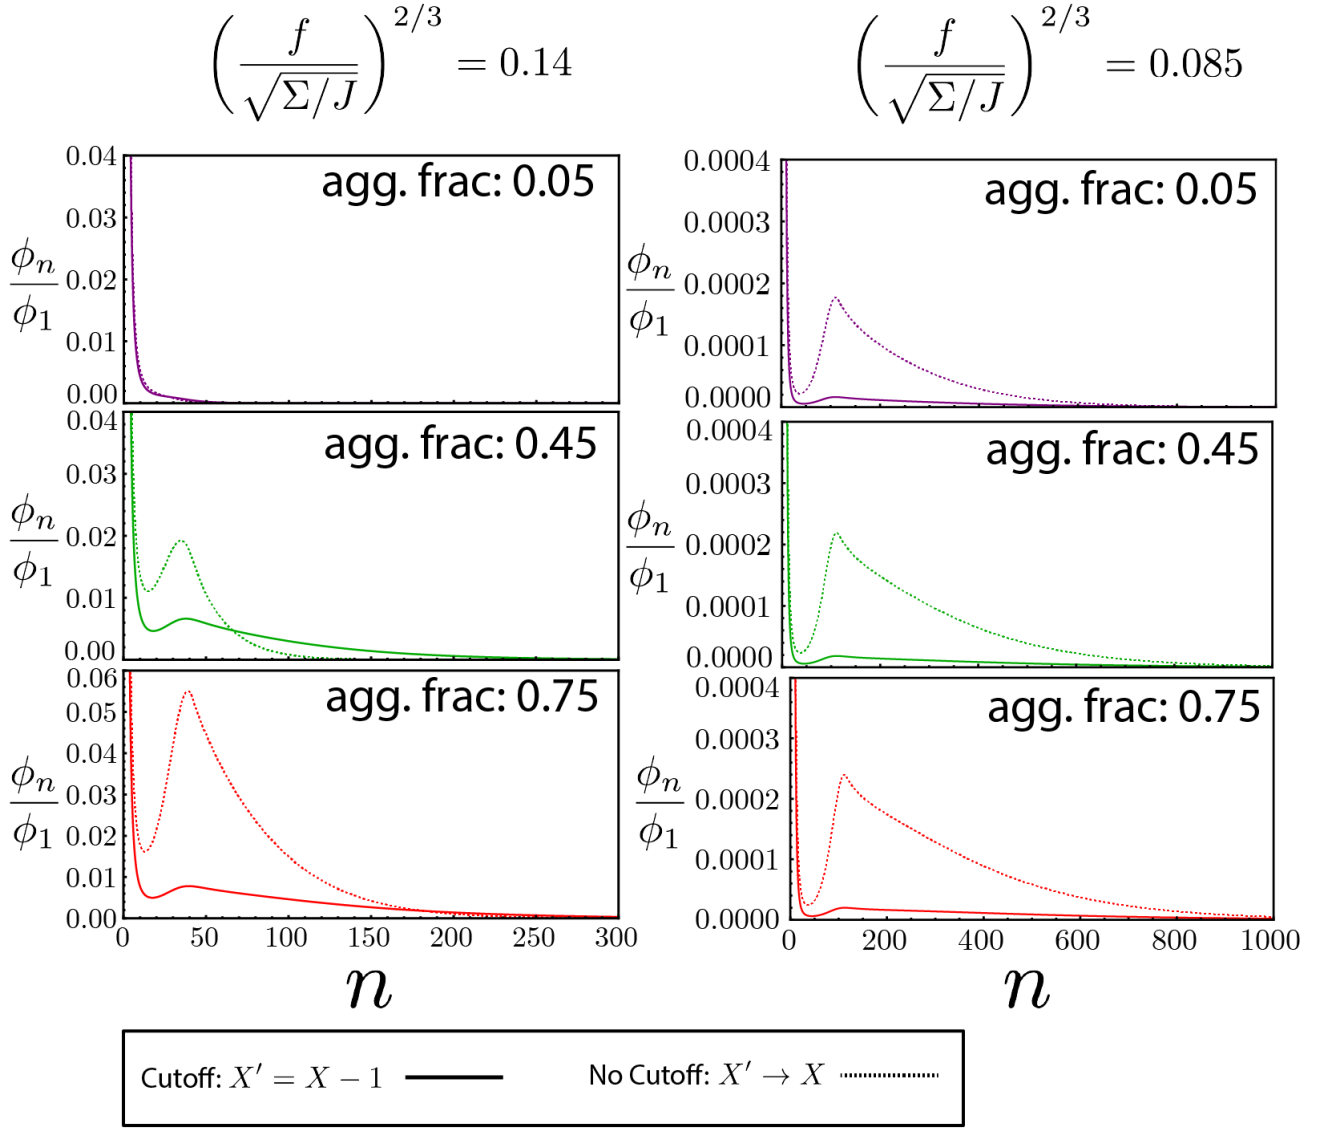

FIG. S4: **Affect of lattice cutoff on aggregate concentration** Comparison of the aggregate concentration, at three different aggregation fractions, computed with the both the cutoff, cutoff-free theory for two different values of  $\ell_d^{-1}$ .

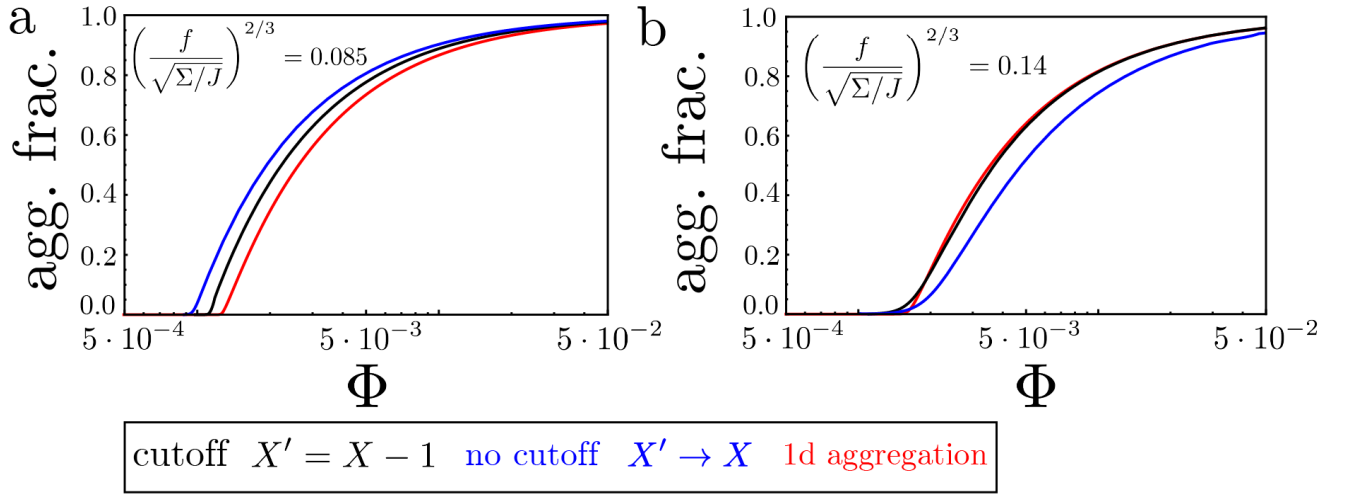

FIG. S5: **Affect of lattice cutoff on aggregation fraction** Comparison of the aggregation fraction computed with the cutoff, cutoff-free and 1d aggregation model for two different values of  $\ell_d^{-1}$ .
